# Supplementary material for: A Large Scale Study of Reader Interactions with Images on Wikipedia
Source: arXiv:2112.01868 source file (2021-12-03)
Supplement: Supplementary file 1 [file Supplementary_Materials_revised.pdf]

# Supplementary Material for A Large Scale Study of Reader Interactions with Images on Wikipedia

Daniele Rama, Tiziano Piccardi, Miriam Redi, Rossano Schifanella

## I. SUPPLEMENTARY FIGURE

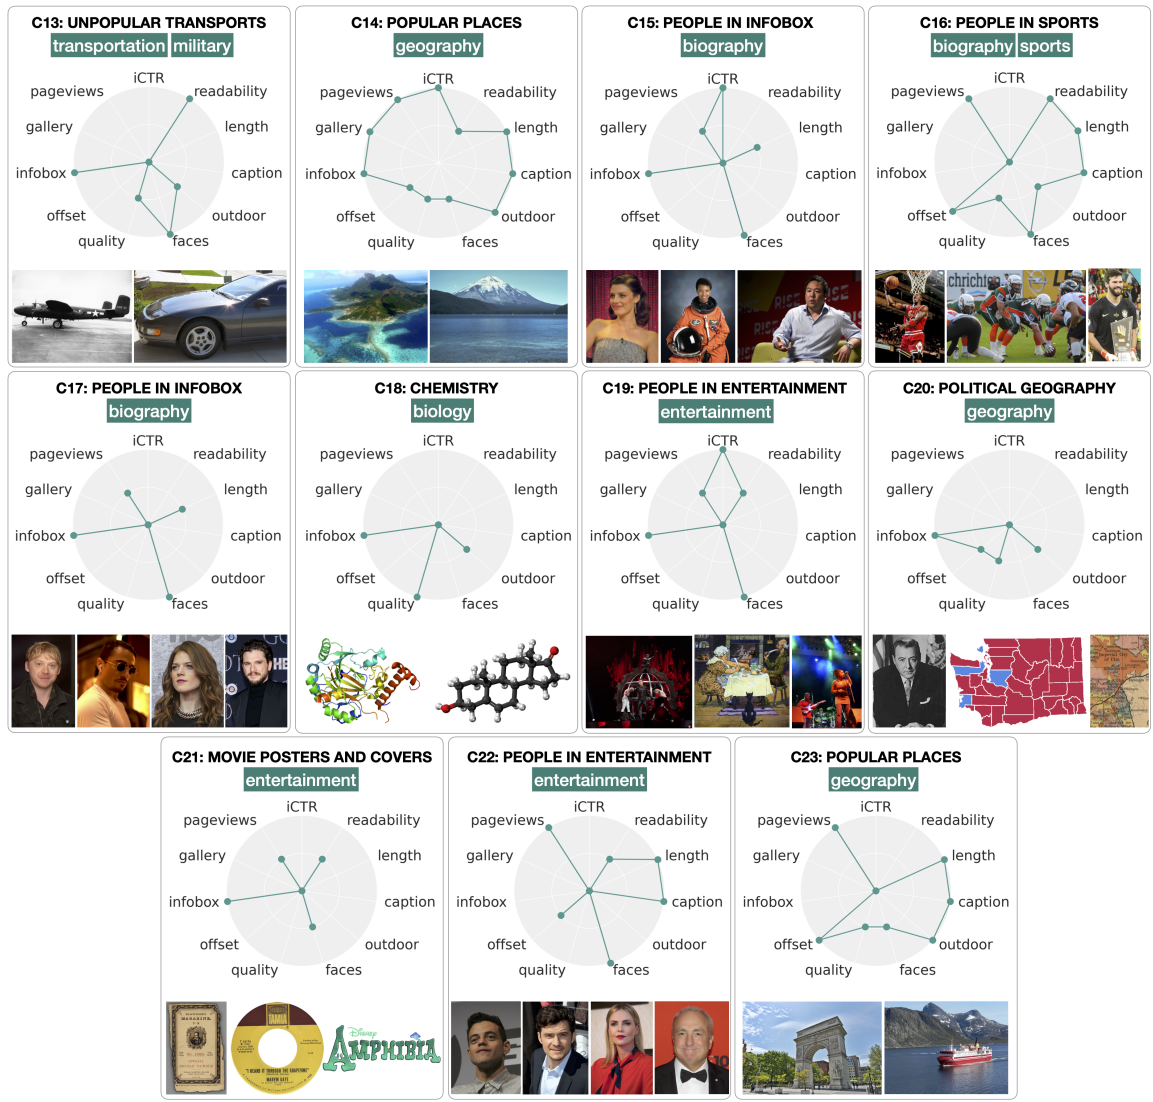

FIG. 1. Visual representation of the clusters not included in the discussion of results in Section 6.3. The radar plots show for a group centroid the intensity of each feature on a 3 classes scale. We summarize in green the topics that cover at least 85% of the images categories in a cluster.

## II. SUPPLEMENTARY TABLE

| Feature              | Correlation with iCTR | Median iCTR | Fraction of images |
|----------------------|-----------------------|-------------|--------------------|
| readability          | 0.110                 |             |                    |
| text length          | -0.308                |             |                    |
| caption              | -0.052                |             |                    |
| offset               | -0.065                |             |                    |
| faces                | -0.142                |             |                    |
| outdoor              | 0.227                 |             |                    |
| quality              | 0.083                 |             |                    |
| resolution           | -0.002                |             |                    |
| popularity (desktop) | 0.175                 |             |                    |
| popularity (mobile)  | 0.211                 |             |                    |
| (placement) infobox  |                       | 0.019       | 0.361              |
| (placement) inline   |                       | 0.016       | 0.483              |
| (placement) gallery  |                       | 0.024       | 0.155              |
| transportation       | 0.181                 | 0.037       | 0.053              |
| visual arts          | 0.167                 | 0.037       | 0.054              |
| engineering          | 0.072                 | 0.027       | 0.024              |
| military             | 0.078                 | 0.025       | 0.047              |
| geography            | 0.166                 | 0.023       | 0.255              |
| environment          | 0.015                 | 0.020       | 0.012              |
| space                | 0.013                 | 0.020       | 0.006              |
| philosophy           | 0.013                 | 0.019       | 0.025              |
| biology              | -0.001                | 0.019       | 0.045              |
| technology           | -0.002                | 0.017       | 0.011              |
| economics            | -0.022                | 0.015       | 0.025              |
| society              | -0.020                | 0.015       | 0.025              |
| food & drink         | -0.013                | 0.015       | 0.008              |
| biography            | -0.104                | 0.014       | 0.155              |
| computer science     | -0.013                | 0.014       | 0.005              |
| history              | -0.051                | 0.012       | 0.029              |
| entertainment        | -0.159                | 0.011       | 0.100              |
| medicine             | -0.035                | 0.011       | 0.009              |
| linguistics          | -0.018                | 0.011       | 0.002              |
| literature           | -0.083                | 0.010       | 0.022              |
| education            | -0.070                | 0.009       | 0.014              |
| math & physics       | -0.027                | 0.009       | 0.002              |
| sports               | -0.146                | 0.008       | 0.050              |
| politics             | -0.101                | 0.008       | 0.022              |

TABLE I. Summary table of (i) the Spearman’s correlation coefficient between the numerical features (including topics) and the target variable, i. e. the image click-through rate, (ii) the median image click-through rate for the categorical feature (*placement*) and the topics, and (iii) the fraction of images by *placement* and topic. All the correlation coefficients are statistically significant with  $p < 0.001$ .
